# Supplementary material for: Fluid Elasticity Can Enable Propulsion at Low Reynolds Number
Source: arXiv:1201.0545 source file (2012-08-20)
Supplement: Supplementary file 1 [file supplemental.pdf]

# Supplementary Material

N.C. Keim, M. Garcia, and P.E. Arratia

January 2, 2012

Two types of fluid are used in the experiments: a viscous Newtonian fluid and a viscoelastic fluid. The Newtonian fluid is a mixture of 4% water (by weight) and 96% pure corn syrup (Cargill "ClearSweet 43/43"). The kinematic viscosity of the Newtonian fluid is approximately 40,000 cSt. The viscoelastic fluid is prepared by adding small amounts of a high-molecular-weight polymer to a viscous Newtonian solvent, in order to minimize the effects of shear-rate-dependent viscosity; this is often called a "Boger fluid." The polymer used here is polyacrylamide (PAA, $M_W = 1 \times 10^6$), which has a flexible backbone. The polymeric solution consists of 0.17% PAA (by mass) in a 93%-corn syrup aqueous solution. Each sample is degassed prior to experiments. To prevent evaporation of water, a layer of mineral oil covers the experimental sample, and coats the free surface of the sample during rheometry.

The polymeric fluid is characterized in a Bohlin "Gemini" strain-controlled rheometer, using a cone-and-plate geometry at a constant temperature of 22 °C. Figure 1 shows that the fluid has a shear viscosity that is nearly constant, with a power-law index of $n = 0.96$; and a pronounced first normal stress difference $N_1$. This behavior is typical of a Boger fluid.

The fluid relaxation time is obtained by fitting the stress relaxation data (Fig. 2) to the generalized linear viscoelastic model of a single relaxation time, of the type $G(t) = G_0 e^{-t/\lambda}$, where $G(t)$ is the fluid shear modulus and $\lambda$ is the longest fluid relaxation time. We find that $\lambda$ is approximately 2 s.

The characteristic strain rate in experiments with dimers ranges from $\sim 0.5$ to 20 $s^{-1}$, depending on $f_{\mathrm{drive}}$. We estimate it from the root-mean-squared of the dimer's angular velocity.

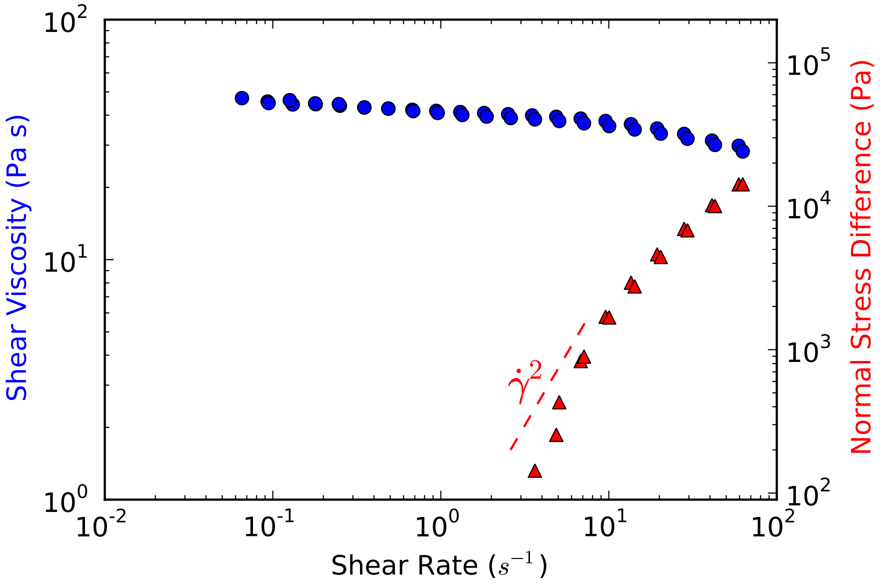


Figure 1: Measurement of shear viscosity (blue circles, left axis) and normal stress difference $N_1$ (red triangles, right axis) under steady shear. Shear rate is ramped down and then up, corresponding to the pairs of symbols. The fluid is weakly shear-thinning; below $\dot{\gamma} \sim 15$ s$^{-1}$ the shear stress magnitude scales as $|\sigma| \propto |\dot{\gamma}|^n$ with $n = 0.96$. A positive first normal stress difference $N_1$ shows scaling consistent with $\dot{\gamma}^2$ below $\dot{\gamma} \sim 15$ s$^{-1}$.

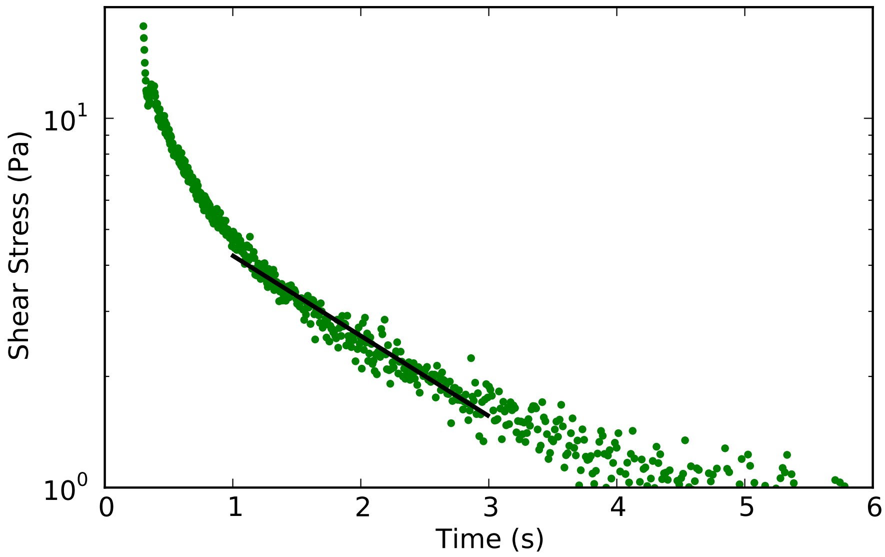


Figure 2: Stress relaxation after a 120% strain step. Solid line represents the longest relaxation time of $\lambda = 2$ s. Results are consistent with those for smaller strain steps.
